# Supplementary material for: Phylogenetic effective sample size
Source: arXiv:1507.07113 source file (2016-05-11)
Supplement: Supplementary file 1 [file Bartoszek_pESS_Supplement.pdf]

# Phylogenetic effective sample size
# Supplementary histograms

Krzysztof Bartoszek

Department of Mathematics, Uppsala University, 751 06 Uppsala, Sweden.
bartoszekkj@gmail.com

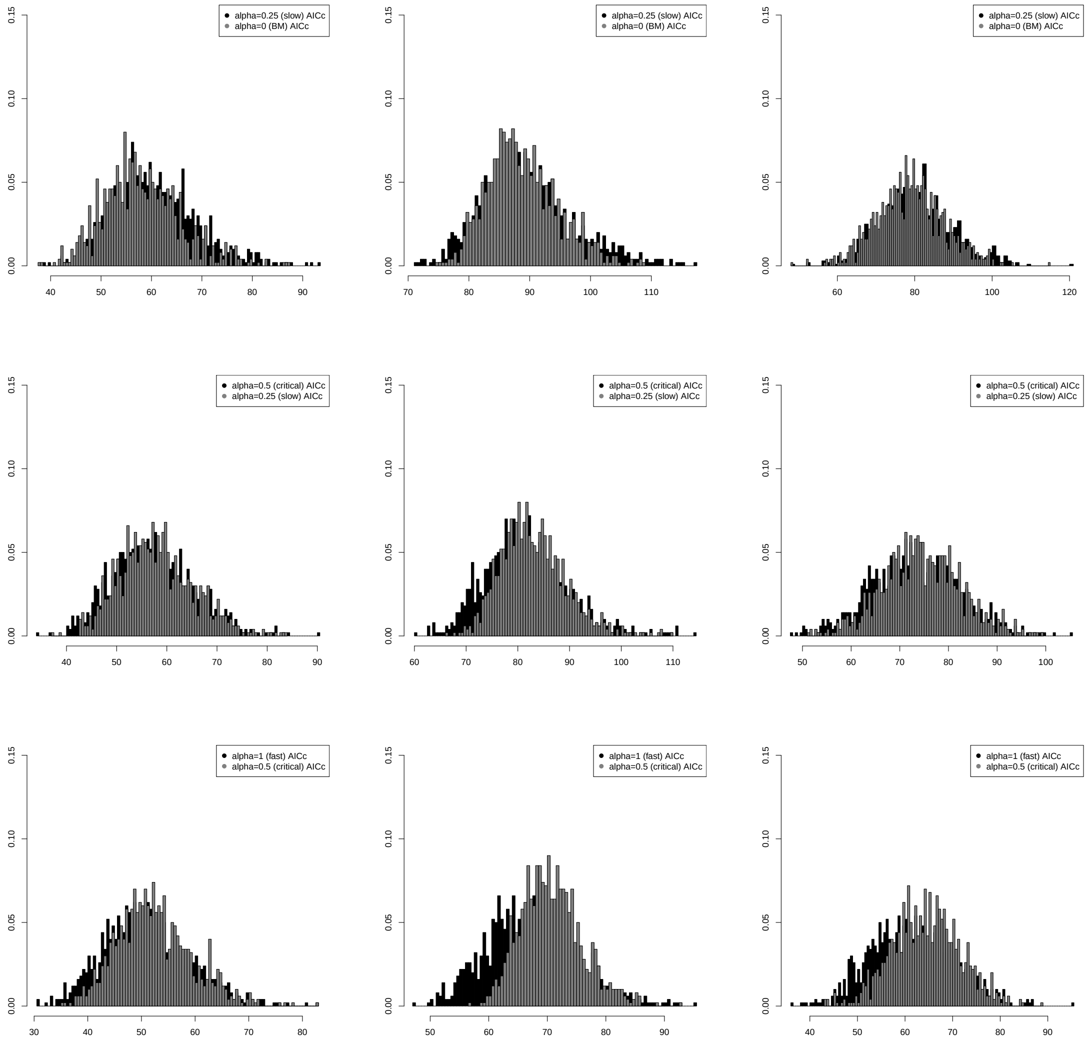


Figure S.1: Histograms of $\text{AIC}_c$ values with $n_e^{MI}$ effective sample size correction for different types of trees and evolutionary processes. The sample sizes are $n = 30$ (left unbalanced tree and Yule) and $n = 32$ (balanced tree). First column: balanced tree, second column: left unbalanced tree, third column: 1000 pure–birth Yule trees ($\lambda = 1$). The balanced trees and unbalanced trees were generated using the function stree() of the R ape package, the Yule trees by the TreeSim R package. First row: Ornstein–Uhlenbeck process ($\alpha = 0.25$, $\sigma^2 = 1$, $X_0 = 0$, $\theta = 0$ black true model), Brownian motion ($X_0 = 0$, $\sigma^2 = 1$ gray alternative model), second row: Ornstein–Uhlenbeck process ($\alpha = 0.5$, $\sigma^2 = 1$, $X_0 = 0$, $\theta = 0$ black true model), Ornstein–Uhlenbeck process ($\alpha = 0.25$, $\sigma^2 = 1$, $X_0 = 0$, $\theta = 0$ gray alternative model), third row: Ornstein–Uhlenbeck process ($\alpha = 1$, $\sigma^2 = 1$, $X_0 = 0$, $\theta = 0$ black true model), fourth row: Ornstein–Uhlenbeck process ($\alpha = 0.5$, $\sigma^2 = 1$, $X_0 = 0$, $\theta = 0$ gray alternative model). We simulate data under both the true and alternative evolutionary models 1000 times and then calculate $\text{AIC}_c$ values for each simulated pair.

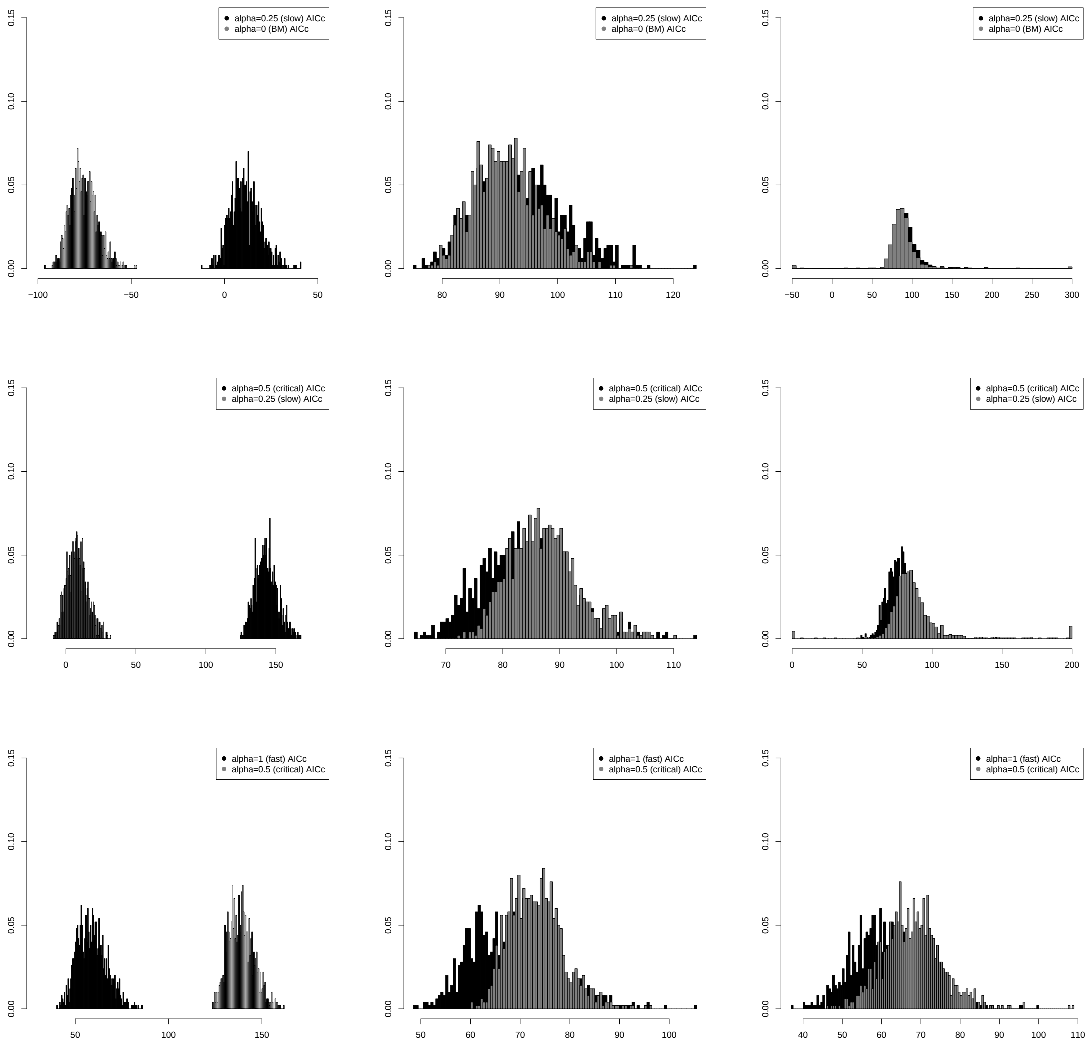


Figure S.2: Histograms of $\text{AIC}_c$ values with $n_e^E$ effective sample size correction for different types of trees and evolutionary processes. The sample sizes are $n = 30$ (left unbalanced tree and Yule) and $n = 32$ (balanced tree). First column: balanced tree, second column: left unbalanced tree, third column: 1000 pure–birth Yule trees ($\lambda = 1$). The balanced trees and unbalanced trees were generated using the function stree() of the R ape package, the Yule trees by the TreeSim R package. First row: Ornstein–Uhlenbeck process ($\alpha = 0.25$, $\sigma^2 = 1$, $X_0 = 0$, $\theta = 0$ black true model), Brownian motion ($X_0 = 0$, $\sigma^2 = 1$ gray alternative model), second row: Ornstein–Uhlenbeck process ($\alpha = 0.5$, $\sigma^2 = 1$, $X_0 = 0$, $\theta = 0$ black true model), Ornstein–Uhlenbeck process ($\alpha = 0.25$, $\sigma^2 = 1$, $X_0 = 0$, $\theta = 0$ gray alternative model), third row: Ornstein–Uhlenbeck process ($\alpha = 1$, $\sigma^2 = 1$, $X_0 = 0$, $\theta = 0$ black true model), fourth row: Ornstein–Uhlenbeck process ($\alpha = 0.5$, $\sigma^2 = 1$, $X_0 = 0$, $\theta = 0$ gray alternative model). We simulate data under both the true and alternative evolutionary models 1000 times and then calculate $\text{AIC}_c$ values for each simulated pair.

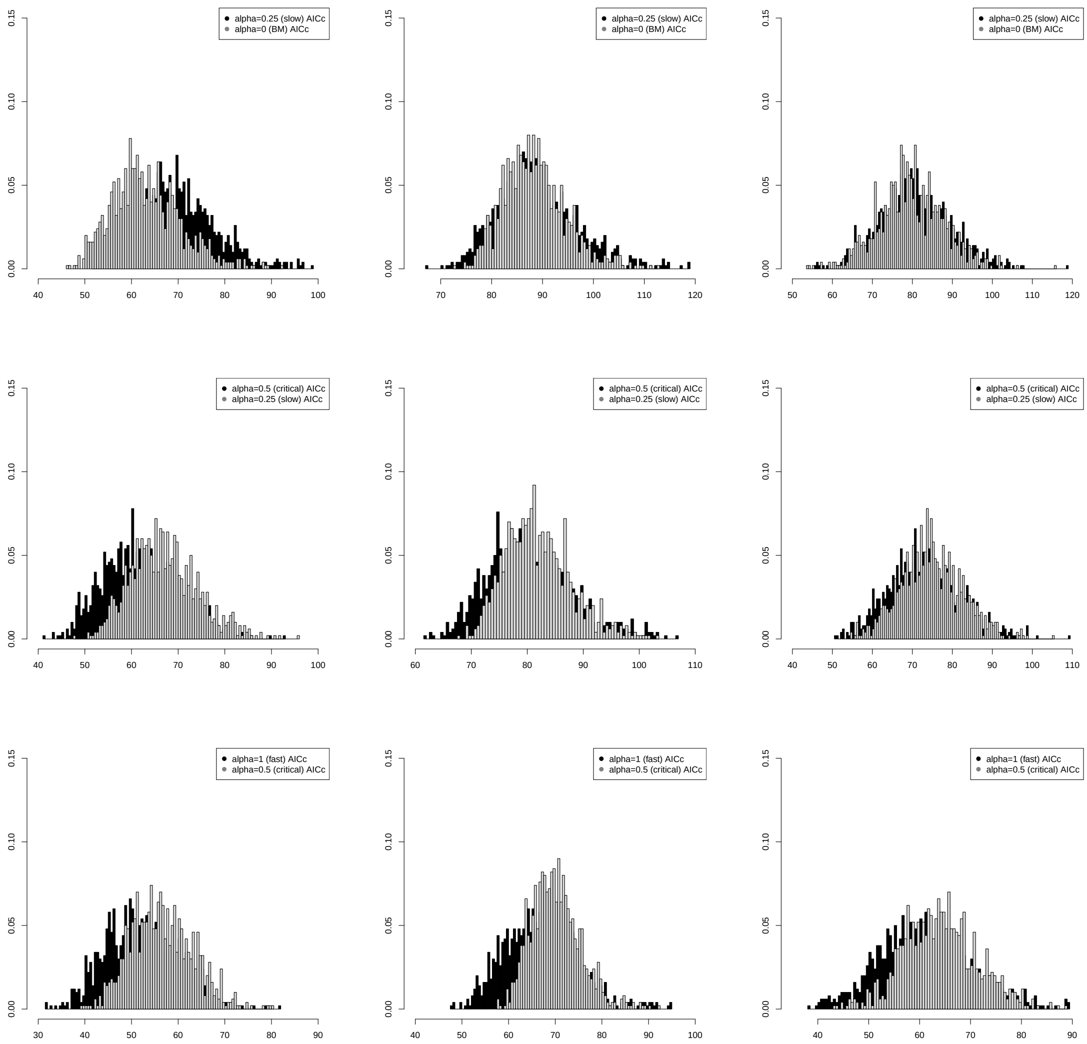


Figure S.3: Histograms of $\mathrm{AIC}_c$ values with $n_e^R$ effective sample size correction for different types of trees and evolutionary processes. The sample sizes are $n = 30$ (left unbalanced tree and Yule) and $n = 32$ (balanced tree). First column: balanced tree, second column: left unbalanced tree, third column: 1000 pure–birth Yule trees ($\lambda = 1$). The balanced trees and unbalanced trees were generated using the function stree() of the R ape package, the Yule trees by the TreeSim R package. First row: Ornstein–Uhlenbeck process ($\alpha = 0.25$, $\sigma^2 = 1$, $X_0 = 0$, $\theta = 0$ black true model), Brownian motion ($X_0 = 0$, $\sigma^2 = 1$ gray alternative model), second row: Ornstein–Uhlenbeck process ($\alpha = 0.5$, $\sigma^2 = 1$, $X_0 = 0$, $\theta = 0$ black true model), Ornstein–Uhlenbeck process ($\alpha = 0.25$, $\sigma^2 = 1$, $X_0 = 0$, $\theta = 0$ gray alternative model), third row: Ornstein–Uhlenbeck process ($\alpha = 1$, $\sigma^2 = 1$, $X_0 = 0$, $\theta = 0$ black true model), fourth row: Ornstein–Uhlenbeck process ($\alpha = 0.5$, $\sigma^2 = 1$, $X_0 = 0$, $\theta = 0$ gray alternative model). We simulate data under both the true and alternative evolutionary models 1000 times and then calculate $\mathrm{AIC}_c$ values for each simulated pair.

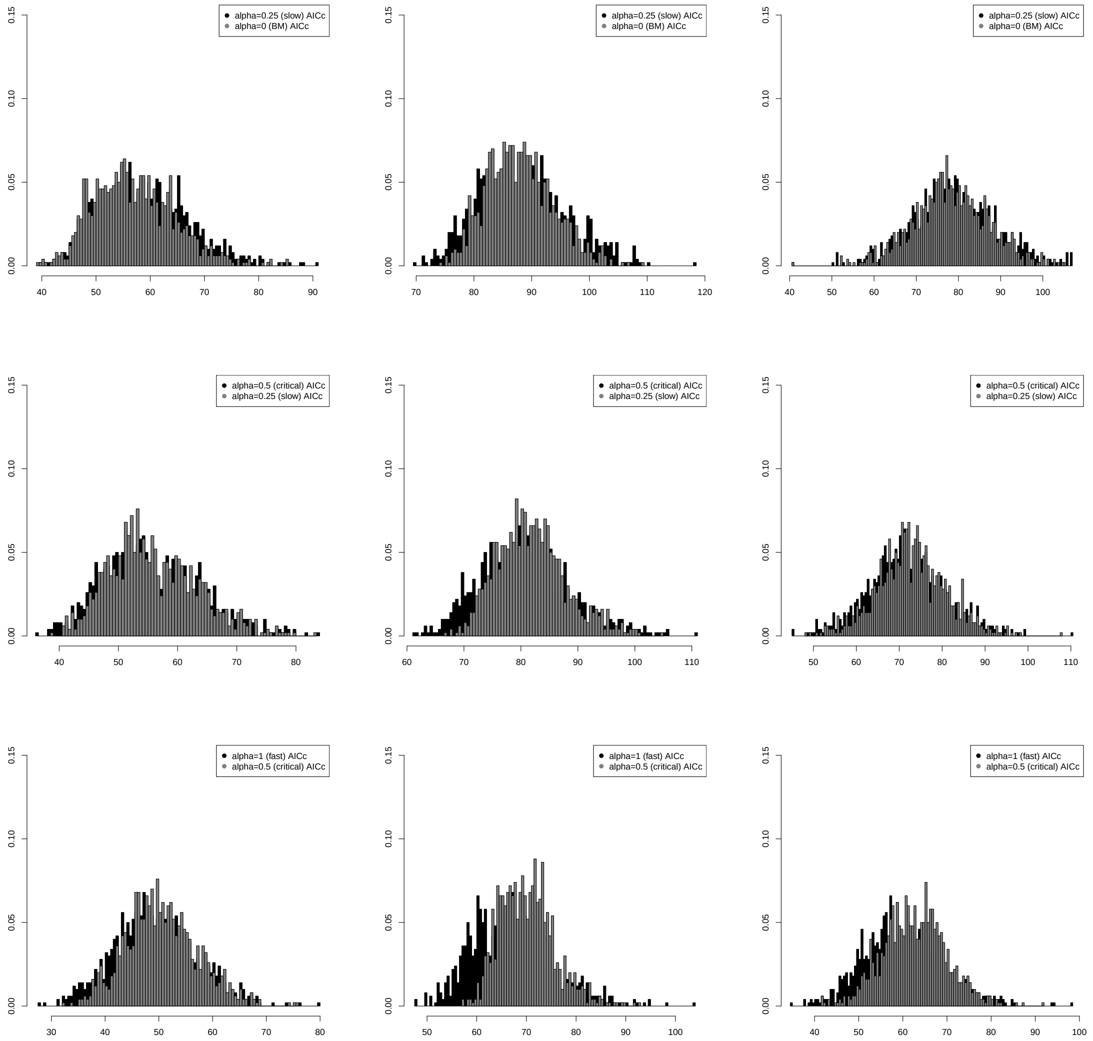


Figure S.4: Histograms of $\mathrm{AIC}_c$ values with no effective sample size correction for different types of trees and evolutionary processes. The sample sizes are $n = 30$ (left unbalanced tree and Yule) and $n = 32$ (balanced tree). First column: balanced tree, second column: left unbalanced tree, third column: 1000 pure–birth Yule trees ($\lambda = 1$). The balanced trees and unbalanced trees were generated using the function stree() of the R ape package, the Yule trees by the TreeSim R package. First row: Ornstein–Uhlenbeck process ($\alpha = 0.25$, $\sigma^2 = 1$, $X_0 = 0$, $\theta = 0$ black true model), Brownian motion ($X_0 = 0$, $\sigma^2 = 1$ gray alternative model), second row: Ornstein–Uhlenbeck process ($\alpha = 0.5$, $\sigma^2 = 1$, $X_0 = 0$, $\theta = 0$ black true model), Ornstein–Uhlenbeck process ($\alpha = 0.25$, $\sigma^2 = 1$, $X_0 = 0$, $\theta = 0$ gray alternative model), third row: Ornstein–Uhlenbeck process ($\alpha = 1$, $\sigma^2 = 1$, $X_0 = 0$, $\theta = 0$ black true model), fourth row: Ornstein–Uhlenbeck process ($\alpha = 0.5$, $\sigma^2 = 1$, $X_0 = 0$, $\theta = 0$ gray alternative model). We simulate data under both the true and alternative evolutionary models 1000 times and then calculate $\mathrm{AIC}_c$ values for each simulated pair.

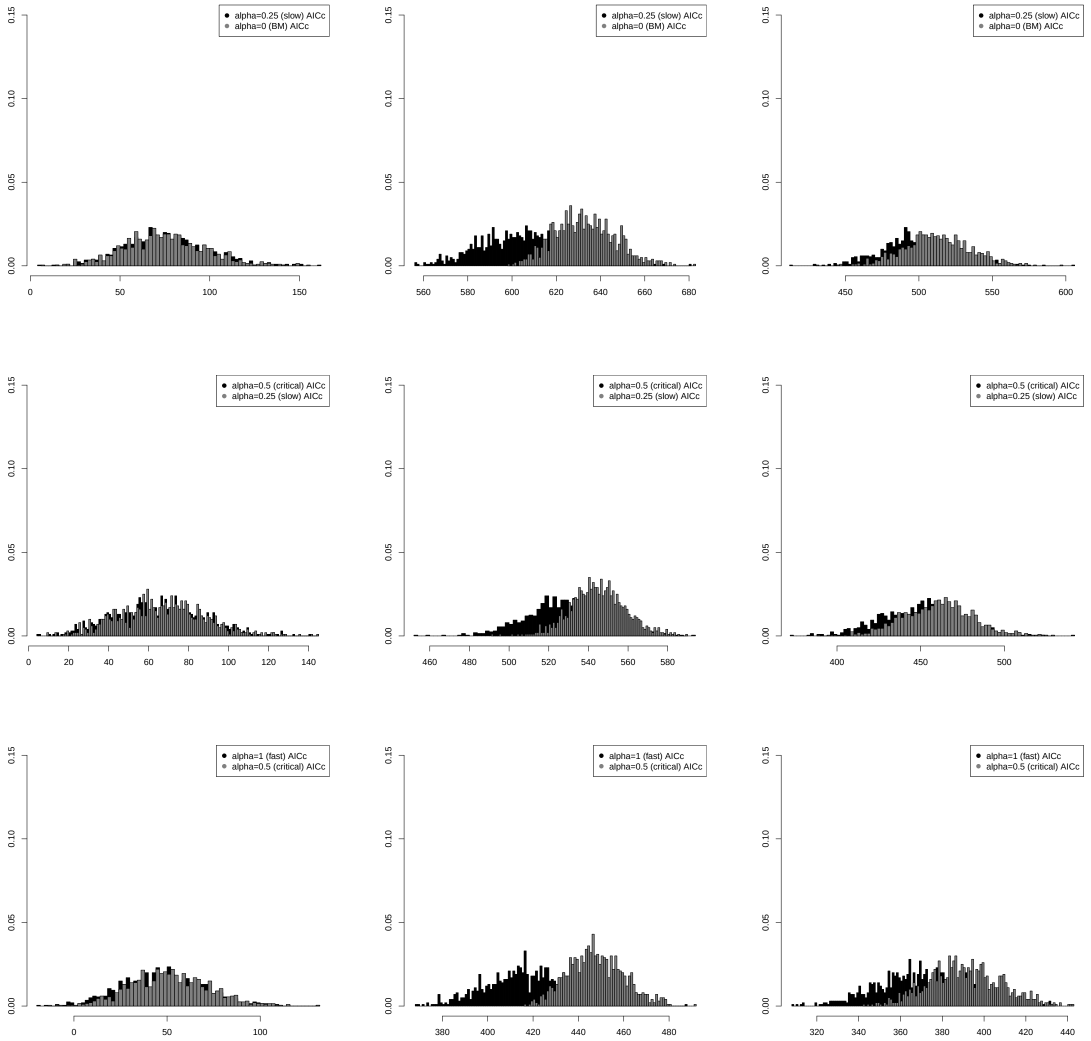


Figure S.5: Histograms of $\text{AIC}_c$ values with $n_e^{MI}$ effective sample size correction for different types of trees and evolutionary processes. The sample sizes are $n = 205$ (left unbalanced tree and Yule) and $n = 256$ (balanced tree). First column: balanced tree, second column: left unbalanced tree, third column: 1000 pure–birth Yule trees ($\lambda = 1$). The balanced trees and unbalanced trees were generated using the function stree() of the R ape package, the Yule trees by the TreeSim R package. First row: Ornstein–Uhlenbeck process ($\alpha = 0.25$, $\sigma^2 = 1$, $X_0 = 0$, $\theta = 0$ black true model), Brownian motion ($X_0 = 0$, $\sigma^2 = 1$ gray alternative model), second row: Ornstein–Uhlenbeck process ($\alpha = 0.5$, $\sigma^2 = 1$, $X_0 = 0$, $\theta = 0$ black true model), Ornstein–Uhlenbeck process ($\alpha = 0.25$, $\sigma^2 = 1$, $X_0 = 0$, $\theta = 0$ gray alternative model), third row: Ornstein–Uhlenbeck process ($\alpha = 1$, $\sigma^2 = 1$, $X_0 = 0$, $\theta = 0$ black true model), fourth row: Ornstein–Uhlenbeck process ($\alpha = 0.5$, $\sigma^2 = 1$, $X_0 = 0$, $\theta = 0$ gray alternative model). We simulate data under both the true and alternative evolutionary models 1000 times and then calculate $\text{AIC}_c$ values for each simulated pair.

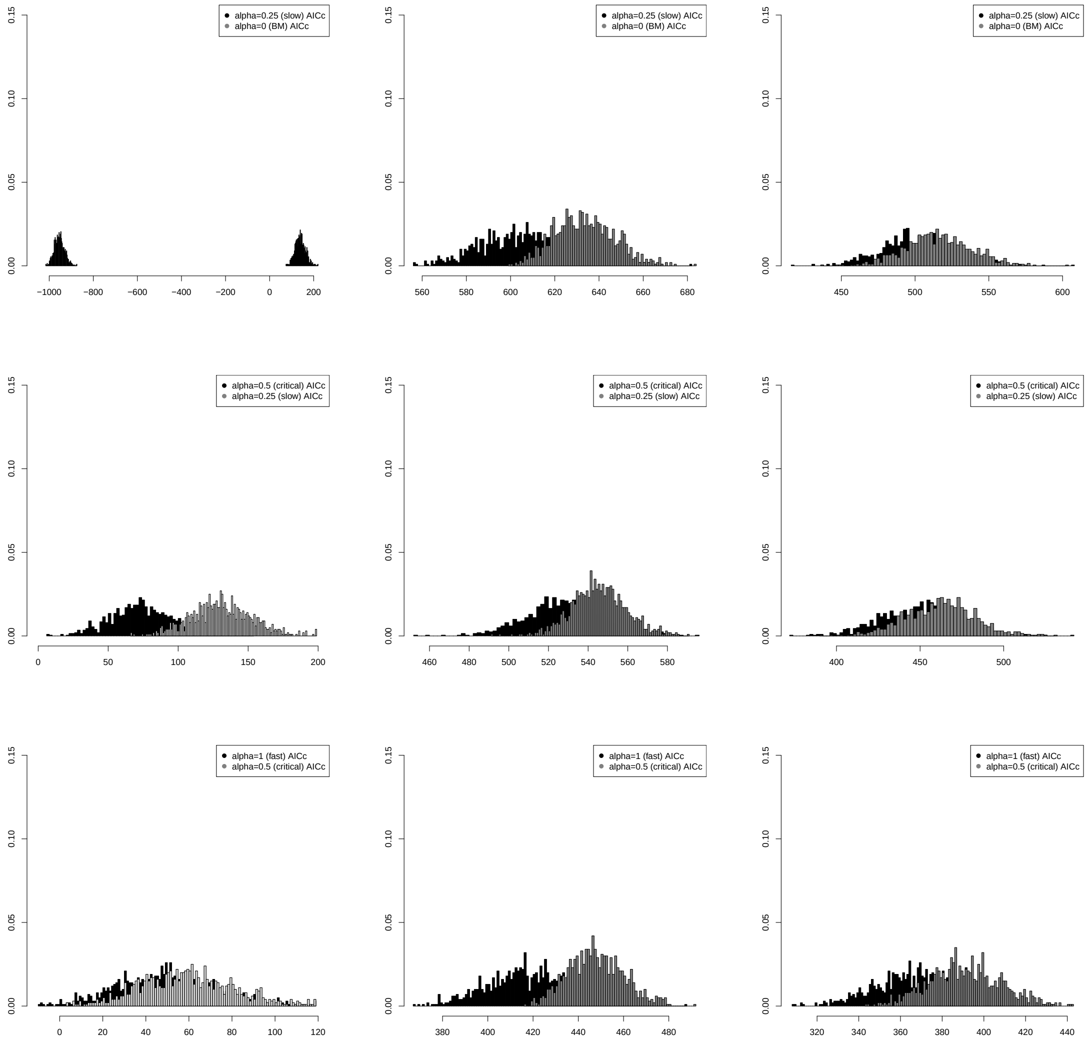


Figure S.6: Histograms of $\text{AIC}_c$ values with $n_e^E$ effective sample size correction for different types of trees and evolutionary processes. The sample sizes are $n = 205$ (left unbalanced tree and Yule) and $n = 256$ (balanced tree). First column: balanced tree, second column: left unbalanced tree, third column: 1000 pure–birth Yule trees ($\lambda = 1$). The balanced trees and unbalanced trees were generated using the function stree() of the R ape package, the Yule trees by the TreeSim R package. First row: Ornstein–Uhlenbeck process ($\alpha = 0.25$, $\sigma^2 = 1$, $X_0 = 0$, $\theta = 0$ black true model), Brownian motion ($X_0 = 0$, $\sigma^2 = 1$ gray alternative model), second row: Ornstein–Uhlenbeck process ($\alpha = 0.5$, $\sigma^2 = 1$, $X_0 = 0$, $\theta = 0$ black true model), Ornstein–Uhlenbeck process ($\alpha = 0.25$, $\sigma^2 = 1$, $X_0 = 0$, $\theta = 0$ gray alternative model), third row: Ornstein–Uhlenbeck process ($\alpha = 1$, $\sigma^2 = 1$, $X_0 = 0$, $\theta = 0$ black true model), fourth row: Ornstein–Uhlenbeck process ($\alpha = 0.5$, $\sigma^2 = 1$, $X_0 = 0$, $\theta = 0$ gray alternative model). We simulate data under both the true and alternative evolutionary models 1000 times and then calculate $\text{AIC}_c$ values for each simulated pair.

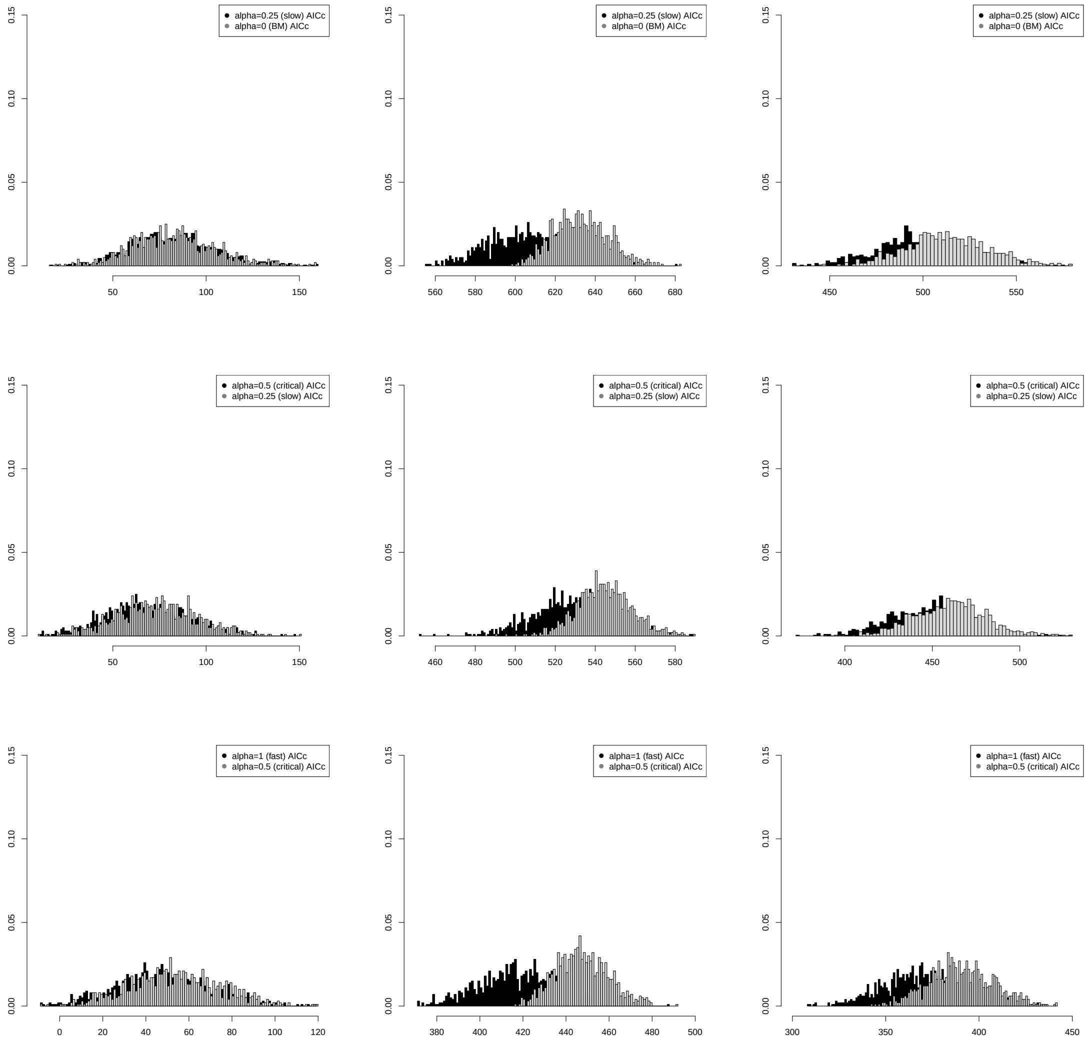


Figure S.7: Histograms of $\text{AIC}_c$ values with $n_e^R$ effective sample size correction for different types of trees and evolutionary processes. The sample sizes are $n = 205$ (left unbalanced tree and Yule) and $n = 256$ (balanced tree). First column: balanced tree, second column: left unbalanced tree, third column: 1000 pure–birth Yule trees ($\lambda = 1$). The balanced trees and unbalanced trees were generated using the function stree() of the R ape package, the Yule trees by the TreeSim R package. First row: Ornstein–Uhlenbeck process ($\alpha = 0.25$, $\sigma^2 = 1$, $X_0 = 0$, $\theta = 0$ black true model), Brownian motion ($X_0 = 0$, $\sigma^2 = 1$ gray alternative model), second row: Ornstein–Uhlenbeck process ($\alpha = 0.5$, $\sigma^2 = 1$, $X_0 = 0$, $\theta = 0$ black true model), Ornstein–Uhlenbeck process ($\alpha = 0.25$, $\sigma^2 = 1$, $X_0 = 0$, $\theta = 0$ gray alternative model), third row: Ornstein–Uhlenbeck process ($\alpha = 1$, $\sigma^2 = 1$, $X_0 = 0$, $\theta = 0$ black true model), fourth row: Ornstein–Uhlenbeck process ($\alpha = 0.5$, $\sigma^2 = 1$, $X_0 = 0$, $\theta = 0$ gray alternative model). We simulate data under both the true and alternative evolutionary models 1000 times and then calculate $\text{AIC}_c$ values for each simulated pair.

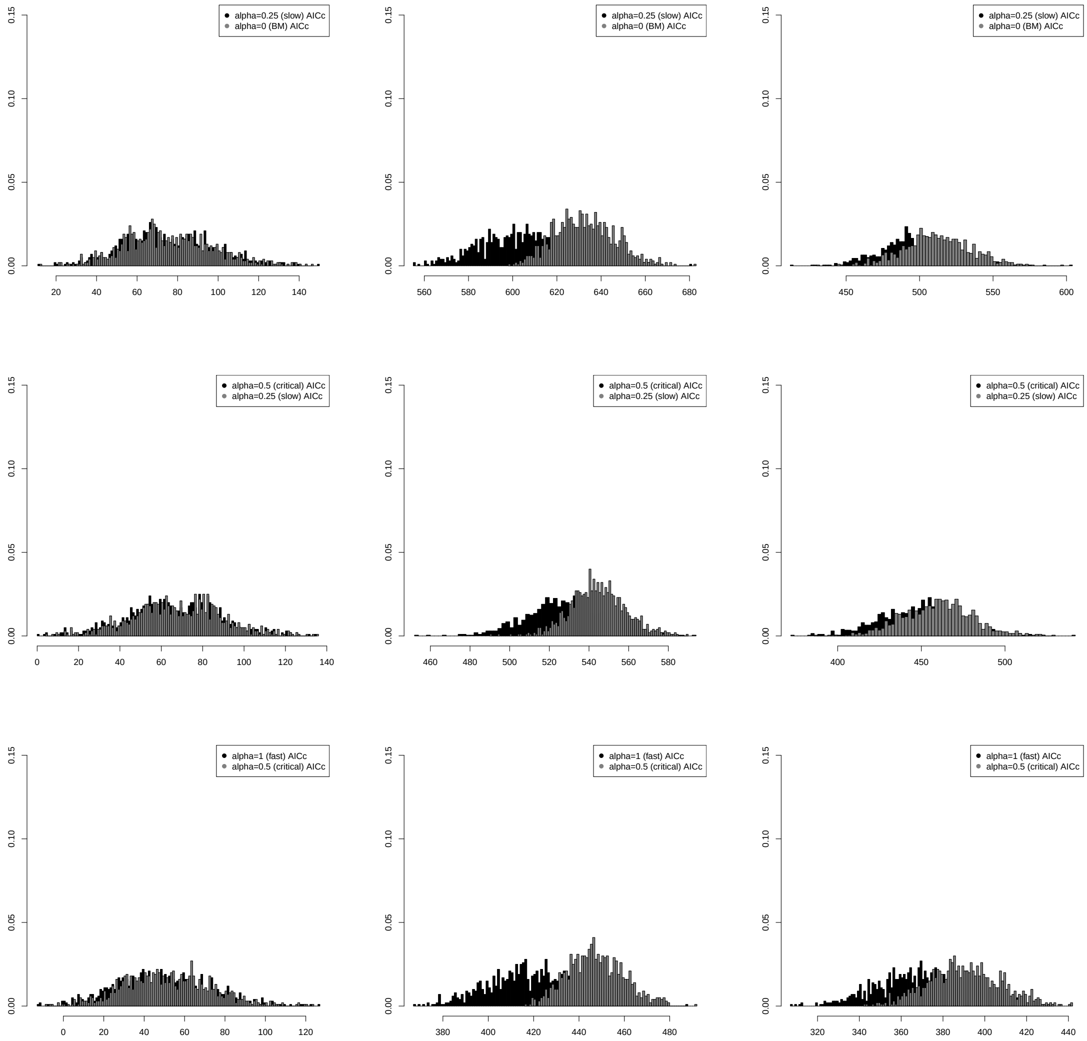


Figure S.8: Histograms of $\mathrm{AIC}_c$ values with no effective sample size correction for different types of trees and evolutionary processes. The sample sizes are $n = 205$ (left unbalanced tree and Yule) and $n = 256$ (balanced tree). First column: balanced tree, second column: left unbalanced tree, third column: 1000 pure–birth Yule trees ($\lambda = 1$). The balanced trees and unbalanced trees were generated using the function stree() of the R ape package, the Yule trees by the TreeSim R package. First row: Ornstein–Uhlenbeck process ($\alpha = 0.25$, $\sigma^2 = 1$, $X_0 = 0$, $\theta = 0$ black true model), Brownian motion ($X_0 = 0$, $\sigma^2 = 1$ gray alternative model), second row: Ornstein–Uhlenbeck process ($\alpha = 0.5$, $\sigma^2 = 1$, $X_0 = 0$, $\theta = 0$ black true model), Ornstein–Uhlenbeck process ($\alpha = 0.25$, $\sigma^2 = 1$, $X_0 = 0$, $\theta = 0$ gray alternative model), third row: Ornstein–Uhlenbeck process ($\alpha = 1$, $\sigma^2 = 1$, $X_0 = 0$, $\theta = 0$ black true model), fourth row: Ornstein–Uhlenbeck process ($\alpha = 0.5$, $\sigma^2 = 1$, $X_0 = 0$, $\theta = 0$ gray alternative model). We simulate data under both the true and alternative evolutionary models 1000 times and then calculate $\mathrm{AIC}_c$ values for each simulated pair.
